# Supplementary material for: Thermodynamic cycles with active matter
Source: arXiv:2002.05932 ancillary file (2020-07-01)
Supplement: Supplementary file 1 [file Supplemental_v4.pdf]

# Supplemental material: Thermodynamic cycles with active matter

Timothy Ekeh, Michael E. Cates, and Étienne Fodor
*DAMTP, Centre for Mathematical Sciences, University of Cambridge, Wilberforce Road, Cambridge CB3 0WA, UK*

## SIMULATION DETAILS

To produce numerical results, we evolved the stochastic differential equations describing Active Brownian Particles (ABPs) using an Euler stepping algorithm in C for both the translational $(x, y)$ and orientational $(\theta)$ degrees of freedom, which we will collectively denote by $\mathbf{Q}$. We discretize the simulation time in units of $\Delta t$ (at most $10^{-4}$) and the simulation time is then $t_i = i\Delta t$ for integer $i$. The coordinates at the start of the time $t_i$ are denoted $\mathbf{Q}(t_i) \equiv \mathbf{Q}_i$

$$\begin{aligned} x_{i+1} &= x_i + F(x_i, \theta_i)\Delta t + \sqrt{2D_\mathrm{t}\Delta t}\,\tilde{\eta}_x, \\ y_{i+1} &= y_i + v\sin\theta\Delta t + \sqrt{2D_\mathrm{t}\Delta t}\,\tilde{\eta}_y, \\ \theta_{i+1} &= \theta_i + \mu_\mathrm{r}\Gamma(\theta_i, x_i)\Delta t + \sqrt{2D_\mathrm{r}\Delta t}\,\tilde{\eta}_\theta, \end{aligned} \tag{1}$$

with $F(x,\theta) = v\cos\theta - \lambda\mu_\mathrm{t}\big[(x-\ell)H(x-\ell) + xH(-x)\big]$ and $\Gamma(\theta, x) = \lambda\kappa\sin(2\theta)\big[H(x-\ell) + H(-x)\big]$. All the $\tilde{\eta}_Q$ are zero-mean unit-variance Gaussian random variables, and we set $\mu_\mathrm{r} = \mu_\mathrm{t} = 1$ in the simulations.

The calculation of observables that are a function of $(x, y, \theta)$ is straightforward. Note that we can write the number density as

$$\begin{aligned} P(\mathbf{Q}_i) &= \sum_{k=1}^{N} \delta(\mathbf{Q}_i^k - \mathbf{Q}_i) \\ &= \sum_{k=1}^{N} \delta(x_i^k - x)\delta(y_i^k - y)\delta(\theta_i^k - \theta). \end{aligned} \tag{2}$$

For a given observable $\mathcal{O}(x(t_i), y(t_i), \theta(t_i))$, the ensemble average is numerically calculated as

$$\langle \mathcal{O}(x(t_i), y(t_i), \theta(t_i)) \rangle = \sum_{k=1}^{N} \mathcal{O}(x_i^k, y_i^k, \theta_i^k). \tag{3}$$

At the start of the simulation, all the particles are randomly distributed within the domain and are left to undergo the stochastic dynamics described by (1) for some initialization time, at least $10^6\Delta t$. The cycle is then implemented by incrementing the control parameters deterministically as

$$\lambda_{i+1} = \lambda_i + \Delta\lambda, \quad \ell_{i+1} = \ell_i + \Delta\ell. \tag{4}$$

For quasistatic calculations, the cycles under investigation are split into many smaller segments. Observables such as work are calculated separately within each segment and then summed to gain the total work output. The steps in $(\ell, \lambda)$ are sufficiently small to assure effective steady state profiles at each stage of the cycle. The color scaling in Fig. 2(b) of the main text follows $(|\mathcal{W}_\mathrm{qs}|/\mathcal{W}_\mathrm{qs})\ln(1 + |\mathcal{W}_\mathrm{qs}|)$. For finite-time cycles, we run the full cycle and collect averages for the extracted work output and dissipated heat. The work output as a function of cycle time is found to obey the form $\mathcal{W} = \mathcal{W}_\mathrm{QS}(1 - \tau_\mathrm{r}/\tau_\mathrm{c})$, with the dimensionless fitting parameter $\tau_\mathrm{r}D_\mathrm{r} = (2.9 \pm 0.4) \times 10^4$ for Fig. 3 in the main text. We report the parameter values for Figs. 2-3 of the main text in Tab. I.

## DEPLETION OF BULK DENSITY

In this Section, we calculate the bulk density which is depleted from the hard wall density $N/\ell$ due to the penetration of particles into the boundary. The precise form is derived in this Section on approximating the position distribution $m_0$ by a Boltzmann factor as $m_0(x) = \rho(\ell, \lambda)\exp\big[-\mu_\mathrm{t}u_\mathrm{t}(x)/(D_\mathrm{t}(1 + \mathrm{Pe}))\big]$, where the bulk density $\rho(\ell, \lambda)$ depends both on $\ell$ and $\lambda$. For harmonic confinement, we get

$$\begin{aligned} N &= \int_{-\infty}^{+\infty} m_0(x)\,\mathrm{d}x \\ &= \rho(\ell, \lambda)\left\{\ell + 2\int_\ell^\infty \exp\left[-\frac{\mu_\mathrm{t}\lambda(x-\ell)^2}{2D_\mathrm{t}(1+\mathrm{Pe})}\right]\mathrm{d}x\right\} \\ &= \rho(\ell, \lambda)\left[\ell + \sqrt{\frac{2\pi D_\mathrm{t}(1+\mathrm{Pe})}{\mu_\mathrm{t}\lambda}}\right], \end{aligned} \tag{5}$$

where we have used the reflection symmetry with respect to the centre of the box, yielding

$$\rho(\ell, \lambda) = \frac{N}{\ell + \sqrt{2\pi D_\mathrm{t}(1+\mathrm{Pe})/(\lambda\mu_\mathrm{t})}}. \tag{6}$$

The number of particles within one wall follows as

$$\int_\ell^\infty m_0\mathrm{d}x = N - \ell\,\rho(\ell, \lambda). \tag{7}$$

## ANGULAR MOMENTS OF THE FOKKER-PLANCK DISTRIBUTION

In this Section, we outline the derivation of the hierarchy of equation for the angular moments defined as

$$m_n(x) = \int_0^{2\pi} \cos(n\theta)\mathcal{P}(x, \theta)\mathrm{d}\theta, \tag{8}$$

TABLE I. Simulation/Plotting parameters for data in Figs. 2-3 of the main text.

| | $D_{\rm t}$ | $v$ | $\mu_{\rm t}, \mu_{\rm r}$ | $D_{\rm r}$ | $\ell_{\rm i}$, $\ell_{\rm f}$ | $\lambda_{\rm i}$, $\lambda_{\rm f}$ | $\kappa$ | $L_y$ | $N$ |
|---|---|---|---|---|---|---|---|---|---|
| Fig. 2(a) | 1 | 6.32 | 1, 1 | 20 | - , - | - , - | 0.2 | 100 | 6000 |
| Fig. 2(b) | 1 | - | 1, 1 | 20 | 20, 40 | 6, 10 | - | 100 | 6000 |
| Figs. 2(c-e) | 5, 15, 30 | 6.32 | 1, 1 | 100 | 40, 50 | 0.3, 0.5 | - | 100 | 6000 |
| Fig. 3 | 4 | 6.32 | 1, 1 | 20 | 20, 40 | 0.3, 0.5 | 40 | 100 | 6000 |

where $\mathcal{P}(x,\theta)$ is the stationary probability density of position $x$ and angle $\theta$. Alternatively, $\mathcal{P}(x,\theta)$ can be written as an even Fourier series:

$$\mathcal{P}(x,\theta) = \frac{1}{2\pi}m_0(x) + \frac{1}{\pi}\sum_{n=1}^{\infty} m_n(x)\cos(n\theta), \tag{9}$$

since the $\sin(n\theta)$ terms, that are odd in angle, have vanishing coefficients by symmetry. Within the wall regions, namely for $x<0$ and $x>\ell$, the full steady-state Fokker-Planck equation for ABPs with harmonic wall confinement is

$$\begin{aligned} 0 = &-\partial_x\big[\big(v\cos\theta - \mu_{\rm t}\partial_x u_{\rm t}\big)\mathcal{P} - D_{\rm t}\partial_x\mathcal{P}\big] \\ &-\partial_\theta\big[\lambda\kappa\mu_{\rm r}\sin(2\theta)\mathcal{P} - D_{\rm r}\partial_\theta\mathcal{P}\big]. \end{aligned} \tag{10}$$

Substituting (9) into (10) and collecting the coefficients of $\cos(n\theta)$ gives the hierarchy of moment equations

$$\begin{aligned} &n^2 D_{\rm r} m_n + \frac{\lambda\kappa\mu_{\rm r} n}{2}(m_{n-2} - m_{n+2}) \\ &= -\partial_x\Big(v\frac{m_{n+1}+m_{n-1}}{2} - \mu_{\rm t} m_n\partial_x u_{\rm t} - D_{\rm t}\partial_x m_n\Big). \end{aligned} \tag{11}$$

Evaluating the $n^{\rm th}$ moment requires deriving all the moments up to $n\pm 2$. Of particular note is the $n=0$ condition, which reads

$$\partial_x\big(v m_1 - \mu_{\rm t} m_0\partial_x u_{\rm t} - D_{\rm t}\partial_x m_0\big) = 0, \tag{12}$$

where we have used that $m_n = m_{-n}$ which follows from the definition of the moments. This is a statement of conserved particle flux. For a confined system, the flux is zero everywhere, which manifests as

$$v m_1 - \mu_{\rm t} m_0\partial_x u_{\rm t} - D_{\rm t}\partial_x m_0 = 0. \tag{13}$$

Furthermore, it is useful to note for the following Sections that all angular moments have definite parity about the centre of the box. Indeed, using $\mathcal{P}(x,\theta) = \mathcal{P}(\ell - x, \pi-\theta)$ we get

$$\begin{aligned} &\int_0^{2\pi}\cos(n\theta)\mathcal{P}(x,\theta)\mathrm{d}\theta \\ &\qquad = \int_0^{2\pi}\cos(n\theta)\mathcal{P}(\ell-x,\pi-\theta)\mathrm{d}\theta \\ &\qquad = \int_\pi^{-\pi}\cos[n(\phi-\pi)]\mathcal{P}(\ell-x,\phi)\mathrm{d}\phi \\ &\qquad = (-1)^n\int_{-\pi}^{\pi}\cos(n\phi)\mathcal{P}(\ell-x,\phi)\mathrm{d}\phi. \end{aligned} \tag{14}$$

In the language of moments, this says that

$$m_n(x) = (-1)^n m_n(\ell - x). \tag{15}$$

All moments are odd or even in space depending on their order. This shows that only the even angular moments are non-zero when integrated over all space, since the odd ones must vanish by symmetry.

To compute explicitly the expression of angular moments integrated over the wall regions, we introduce angular functions $f_\pm(\theta)$ by integrating $\mathcal{P}$ in (9) over the right wall ($x:\ell\to\infty$) and the left wall ($x:-\infty\to 0$), respectively, yielding

$$\begin{aligned} f_\pm(\theta) = &\frac{1}{2\pi}\int_\ell^\infty m_0\mathrm{d}x \\ &+\frac{1}{\pi}\sum_{n=1}^{\infty}(\pm 1)^n\cos(n\theta)\int_\ell^\infty m_n\mathrm{d}x. \end{aligned} \tag{16}$$

Note that for $f_-(\theta)$ we have used (15) to redefine the integration range. We then integrate the Fokker-Plank equation (10) to the right and left of the box in the same way, yielding two differential equations:

$$\begin{aligned} 0 &= v\cos\theta\,\mathcal{P}(\ell,\theta) + D_{\rm r}\partial_\theta^2 f_+ - \mu_{\rm r}\partial_\theta(\Gamma f_+), \\ 0 &= -v\cos\theta\,\mathcal{P}(0,\theta) + D_{\rm r}\partial_\theta^2 f_- - \mu_{\rm r}\partial_\theta(\Gamma f_-). \end{aligned} \tag{17}$$

Next, we define the symmetric/antisymmetric linear combinations $F_\pm = (f_-\pm f_+)/2$, which satisfy the equations

$$0 = \frac{1}{2}v\cos\theta\big[\mathcal{P}(\ell,\theta)\mp\mathcal{P}(0,\theta)\big] + D_{\rm r}\partial_\theta^2 F_\pm - \mu_{\rm r}\partial_\theta(\Gamma F_\pm). \tag{18}$$

To provide an explicit solution for $F_\pm$, we assume that the distribution is flat everywhere outside of the wall region, so that $\mathcal{P}(x,\theta) = \rho(\ell,\lambda)/(2\pi)$ within the bulk, which formally neglects any effects due to boundary accumulation provided that the rotational diffusion coefficient is large enough ($D_{\rm r}\gg\lambda\mu_{\rm t}$). The equations for $F_\pm$ then simplify to

$$\begin{aligned} 0 &= D_{\rm r}\partial_\theta F_+ - \mu_{\rm r}\Gamma F_+, \\ 0 &= \frac{v\rho(\ell,\lambda)}{2\pi}\sin\theta + D_{\rm r}\partial_\theta F_- - \mu_{\rm r}\Gamma F_-, \end{aligned} \tag{19}$$

yielding

$$F_+ = A\exp\Big[\frac{\mu_{\rm r}}{D_{\rm r}}\int^\theta\Gamma(\theta')\mathrm{d}\theta'\Big] = A\exp\Big[-\frac{\lambda_\kappa}{2}\cos(2\theta)\Big], \tag{20}$$

where $A$ is determined through normalisation. From (15-16), we get

$$\int_0^{2\pi} F_+(\theta)\mathrm{d}\theta = \frac{1}{2}\left[\int_\ell^\infty m_0\mathrm{d}x + \int_{-\infty}^0 m_0\mathrm{d}x\right] = \int_\ell^\infty m_0\mathrm{d}x. \tag{21}$$

Using this condition, we derive the full solution for $F_+$:

$$F_+(\theta) = \frac{2\exp(-\lambda_\kappa\cos(2\theta)/2)}{\pi I_0(\lambda_\kappa/2)}\int_\ell^\infty m_0\mathrm{d}x, \tag{22}$$

where $I_n(x)$ is the modified Bessel function of the first kind. The integral over even angular moments then come from calculating the Fourier coefficients of $F_+$:

$$\int_\ell^\infty m_{2n}\mathrm{d}x = \int_0^{2\pi} F_+(\theta)\cos(2n\theta)\mathrm{d}\theta = (-1)^n\frac{I_n(\lambda_\kappa/2)}{I_0(\lambda_\kappa/2)}\int_\ell^\infty m_0\mathrm{d}x. \tag{23}$$

Similarly, the expression for $F_-$ follows by solving (19):

$$F_-(\theta) = -\frac{v\rho(\ell,\lambda)}{2D_\mathrm{r}}\sqrt{\frac{\pi}{\lambda_\kappa}}\,\mathrm{e}^{-\lambda_\kappa[1+\cos(2\theta)]/2}\mathrm{erfi}\big[\sqrt{\lambda_\kappa}\cos\theta\big], \tag{24}$$

where we have used the boundary condition $F_-(\pi/2) = 0$ deduced from (15-16), and the "imaginary error function" is defined by

$$\mathrm{erfi}(x) = \frac{2}{\sqrt{\pi}}\int_0^x \mathrm{e}^{y^2}\mathrm{d}y. \tag{25}$$

The integral over odd angular moments is then given by

$$\int_\ell^\infty m_{2n+1}\mathrm{d}x = \int_0^{2\pi} F_-(\theta)\cos[(2n+1)\theta]\mathrm{d}\theta = -\frac{v\rho(\ell,\lambda)}{D_\mathrm{r}}\sqrt{\frac{\pi}{\lambda_\kappa}}\int_0^\pi \cos[(2n+1)\theta] \times \mathrm{e}^{-\lambda_\kappa(1+\cos(2\theta))/2}\mathrm{erfi}\big[\sqrt{\lambda_\kappa}\cos\theta\big]\mathrm{d}\theta. \tag{26}$$

At $n = 0$, this integral can be done exactly to obtain the function $\phi$ defined in (5) of the main text, and which has been calculated in prior work by Solon *et al.* (Ref. [30] in main text) through a different method.

## AVERAGE POTENTIAL ENERGIES

In this Section, we derive the expression for $\psi$ and $\chi$ which appear in the average confining and aligning potential energies, see (7) of main text. To this end, we calculate the energy in the right hand wall only, and then obtain the energy for the entire system by doubling the answer. It is convenient for the following calculations to define two dimensionless parameters, both of which are scaled wall stiffnesses:

$$\lambda_t = \lambda\mu_\mathrm{t}/D_\mathrm{r}, \quad \lambda_\kappa = \lambda\mu_\mathrm{r}\kappa/D_\mathrm{r}. \tag{27}$$

Denoting the confining potential energy in the right hand wall as $\langle u_\mathrm{t}\rangle_r$, we can write that

$$\langle u_\mathrm{t}\rangle_r = \int_\ell^\infty m_0(x)u_\mathrm{t}(x)\mathrm{d}x, \tag{28}$$

and, for a harmonic potential $u_\mathrm{t}\propto(x-\ell)^2$, we get

$$\langle u_\mathrm{t}\rangle_r = \int_\ell^\infty m_0\frac{x-\ell}{2}\partial_x u_\mathrm{t}\mathrm{d}x. \tag{29}$$

Using (13), we then deduce

$$\langle u_\mathrm{t}\rangle_r = \frac{1}{\mu_t}\int_\ell^\infty\big(vm_1 - D_\mathrm{t}\partial_x m_0\big)\frac{x-\ell}{2}\mathrm{d}x = \frac{v}{2\mu_t\lambda}\int_\ell^\infty m_1\partial_x u_\mathrm{t}\mathrm{d}x - \frac{D_\mathrm{t}}{2\mu_t\lambda}\int_\ell^\infty(\partial_x m_0)\partial_x u_\mathrm{t}\mathrm{d}x, \tag{30}$$

and after integrating the last term by parts we get

$$\langle u_\mathrm{t}\rangle_r = \frac{v}{2\mu_t\lambda}\int_\ell^\infty m_1\partial_x u_\mathrm{t}\mathrm{d}x + \frac{D_\mathrm{t}}{2\mu_\mathrm{t}}\int_\ell^\infty m_0\mathrm{d}x. \tag{31}$$

Thus, we need to evaluate the integral $\int m_1\partial_x u_\mathrm{t}\mathrm{d}x$.

To this end, we introduce the angular functions $g_\pm(\theta)$ defined by

$$g_\pm(\theta) = \pm\frac{1}{2\pi}\int_\ell^\infty m_0\partial_x u_t\mathrm{d}x + \frac{1}{\pi}\sum_{n=1}^\infty(\pm1)^{n+1}\cos(n\theta)\int_\ell^\infty m_n\partial_x u_\mathrm{t}\mathrm{d}x. \tag{32}$$

We multiply (10) by $\partial_x u_\mathrm{t}$ and integrate over $x$ to get

$$D_\mathrm{r}\partial_\theta^2 g_\pm - \mu_\mathrm{r}\partial_\theta(\Gamma g_\pm) + \lambda v\cos\theta f_\pm - \lambda\mu_\mathrm{t}g_\pm = \mp\lambda D_\mathrm{t}\mathcal{P}(0,\theta), \tag{33}$$

where $f_\pm$ is defined in (16). We define $G_+ = (g_+ + g_-)/2$, so that

$$G_+(\theta) = \frac{1}{\pi}\sum_{n=0}^\infty\cos[(2n+1)\theta]\int_\ell^\infty m_{2n+1}\partial_x u_\mathrm{t}\mathrm{d}x. \tag{34}$$

Therefore, evaluating $G_+$ and taking its first Fourier coefficient allows one to evaluate $\int m_1\partial_x u_\mathrm{t}\mathrm{d}x$:

$$\int_\ell^\infty m_1\partial_x u_\mathrm{t}\mathrm{d}x = \int_0^{2\pi} G_+(\theta)\cos\theta\,\mathrm{d}\theta. \tag{35}$$

From (33), we deduce that $G_+$ satisfies the equation:

$$D_\mathrm{r}\partial_\theta^2 G_+ - \mu_\mathrm{r}\partial_\theta(\Gamma G_+) - \lambda\mu_\mathrm{t}G_+ = -\lambda v\cos\theta F_+. \tag{36}$$

The solution can be written implicitly in terms of the Green's function $\mathcal{G}$ satisfying

$$\partial_\theta^2\mathcal{G} - \lambda_\kappa\partial_\theta\big[\sin(2\theta)\,\mathcal{G}\big] = \delta(\theta-\zeta), \tag{37}$$

so that

$$G_+(\eta_1) = \lambda_t \int_0^{2\pi} \mathcal{G}(\eta_1,\eta_2)\left[G_+(\eta_2) - \frac{v\cos\eta_2}{\mu_\mathrm{t}} F_+(\eta_2)\right]\mathrm{d}\eta_2. \tag{38}$$

When considering the first Fourier component of $G_+$ as in (35), we get

$$\begin{aligned}\int_\ell^\infty m_1 \partial_x u_\mathrm{t} \mathrm{d}x = \lambda_t \int_0^{2\pi} \cos\eta_1 \mathcal{G}(\eta_1,\eta_2)\mathrm{d}\eta_1\mathrm{d}\eta_2 \\ \times\left[G_+(\eta_2) - \frac{v\cos\eta_2}{\mu_\mathrm{t}} F_+(\eta_2)\right].\end{aligned} \tag{39}$$

To proceed further, we assume that the Green's function $\mathcal{G}$ can be written as

$$\mathcal{G}(\eta_1,\eta_2) = \frac{1}{\pi}\sum_{m=1}^{\infty} \tilde{\mathcal{G}}_m \cos[m(\eta_1-\eta_2)], \tag{40}$$

with constant coefficients $\tilde{\mathcal{G}}_m$. This is not true generically since (37) is not translationally invariant with respect to $\theta$. Hence, we expect the approximate form (40) to hold for small $\lambda\mu_r\kappa/D_r$, as this parameter controls the strength of the term breaking translational invariance in (37). Substituting (40) in (39), we integrate over angles to get

$$\begin{aligned}\int_\ell^\infty m_1 \partial_x u_\mathrm{t} \mathrm{d}x = \lambda_t \tilde{\mathcal{G}}_1 \int \mathrm{d}\eta \cos\eta G_+(\eta) \\ - \frac{v}{\mu_\mathrm{t}} \lambda_t \tilde{\mathcal{G}}_1 \int_0^{2\pi} \cos^2(\eta) F_+(\eta)\mathrm{d}\eta.\end{aligned} \tag{41}$$

Noting that the first integral on the right hand side is again the first Fourier coefficient of $G_+$, we obtain

$$\begin{aligned}&\int_\ell^\infty m_1 \partial_x u_\mathrm{t} \mathrm{d}x \\ &= \frac{v}{\mu_\mathrm{t}} \frac{\lambda_t \tilde{\mathcal{G}}_1(\lambda_\kappa)}{\lambda_t \tilde{\mathcal{G}}_1(\lambda_\kappa) - 1} \int_0^{2\pi} \cos^2(\eta) F_+(\eta)\mathrm{d}\eta \\ &= \frac{v}{2\mu_\mathrm{t}} \frac{\lambda_t \tilde{\mathcal{G}}_1(\lambda_\kappa)}{\lambda_t \tilde{\mathcal{G}}_1(\lambda_\kappa) - 1}\left[1 - \frac{I_1(\lambda_\kappa/2)}{I_0(\lambda_\kappa/2)}\right] \int_\ell^\infty m_0 \mathrm{d}x,\end{aligned} \tag{42}$$

where we have used (22). It now remains to evaluate $\tilde{\mathcal{G}}_1$.

In what follows, we show that $\tilde{\mathcal{G}}_1 = -\phi(\lambda_\kappa)$ where the function $\phi(z) = (1-\mathrm{e}^{-z})/z$ appears in (5) of the main text. The mechanical pressure $P$ is defined as

$$\begin{aligned}P &= \int_\ell^\infty m_0 \partial_x u_\mathrm{t} \mathrm{d}x \\ &= \frac{v}{\mu_\mathrm{t}} \int_\ell^\infty m_1 \mathrm{d}x + \frac{D_\mathrm{t}}{\mu_\mathrm{t}} \rho(\ell,\lambda),\end{aligned} \tag{43}$$

where we have used (13). Comparing (43) with (5) of the main text, we deduce

$$\int_\ell^\infty m_1 \mathrm{d}x = \frac{v\rho(\ell,\lambda)}{2D_\mathrm{r}} \phi(\lambda_\kappa). \tag{44}$$

The function $F_-$ satisfies the differential equation (19) whose solution can be written in terms of $\mathcal{G}$ as

$$F_-(\theta) = -\frac{v\rho(\ell,\lambda)}{2\pi D_\mathrm{r}} \int_0^{2\pi} \mathcal{G}(\theta,\eta)\cos\eta\,\mathrm{d}\eta. \tag{45}$$

Taking the first Fourier coefficient of $F_-$ then provides access to $\int m_1(x)\mathrm{d}x$ as

$$\begin{aligned}\int_\ell^\infty m_1(x)\mathrm{d}x &= \int_0^{2\pi} F_-(\theta)\cos\theta\mathrm{d}\theta \\ &= -\frac{v\rho(\ell,\lambda)}{2\pi D_\mathrm{r}} \iint \mathcal{G}(\theta,\eta)\cos\theta\cos\eta\,\mathrm{d}\theta\mathrm{d}\eta \\ &= -\frac{v\rho(\ell,\lambda)}{2D_\mathrm{r}} \tilde{\mathcal{G}}_1,\end{aligned} \tag{46}$$

from which $\tilde{\mathcal{G}} = -\phi(\lambda_\kappa)$ follows using (44). Then, using (31) and (42), the average confining potential energy reads

$$\begin{aligned}\langle u_\mathrm{t}\rangle &= \frac{D_\mathrm{t}}{\mu_\mathrm{t}}(1 + \mathrm{Pe}\,\psi)\int_\ell^\infty m_0 \mathrm{d}x, \\ \psi &= \frac{\phi(\lambda_\kappa)}{1 + \lambda_t\,\phi(\lambda_\kappa)}\left[1 - \frac{I_1(\lambda_\kappa/2)}{I_0(\lambda_\kappa/2)}\right],\end{aligned} \tag{47}$$

as presented in (7) of the main text.

Finally, the average aligning potential energy is defined as

$$\langle u_\mathrm{r}\rangle = \frac{\lambda\kappa}{2}\langle\cos(2\theta)[H(-x) + H(x-\ell)]\rangle, \tag{48}$$

which follows directly from (23) as

$$\langle u_\mathrm{r}\rangle = -\frac{\lambda\kappa\chi}{2}\int_\ell^\infty m_0 \mathrm{d}x, \quad \chi = \frac{I_1(\lambda_\kappa/2)}{I_0(\lambda_\kappa/2)}, \tag{49}$$

as presented in (7) of the main text.
